# Supplementary material for: A termination criterion for stochastic gradient descent for binary classification
Source: arXiv:2003.10312 source file (2020-03-23)
Supplement: Supplementary file 1 [file arxiv_appendix.tex]

\section{Appendix}
In this section, we provide proofs of technical results that we used in the paper.
\subsection{Drift Analysis Lemma}
Here we state and prove a result on Drift Analysis that we used in the paper. Recall that we require the following equation to hold 
\begin{equation}\label{drift_equation1_appendix}
  \left( \bE\left[V(\btheta_k)|\mathcal{F}_{k-1} \right]-V(\btheta_{k-1}) \right)1_{\{\btheta_{k-1}\not\in C\}}\leq -1_{\{\btheta_{k-1}\not\in C\}}.
\end{equation}
However, when the iterate lies inside $C$, then we do not assume any bound on the expected increase in the drift function. Nevertheless, when the target set $C$ is compact then there exists a positive constant $b>0$ such that 
\begin{equation}\label{drift_equation2_appendix}
  \left( \bE\left[V(\btheta_k)|\mathcal{F}_{k-1} \right]-V(\btheta_{k-1}) \right)1_{\{\btheta_{k-1}\in C\}}\leq b1_{\{\btheta_{k-1}\in C\}},
\end{equation}
The following lemma bounds the expected value of return times $\tau_m^C$.  
\begin{lemma}\label{lem:drift_lemma_appendix} Suppose that for some test function $V$ and a target set $C$, the drift equation \eqref{drift_equation1_appendix} holds. Let $\hat{\btheta} \in \R^d\backslash C$. The following is then true
\begin{equation}
    \bE[\tau_1^C|\btheta_0=\hat{\btheta}]\leq V(\hat{\btheta}).
\end{equation}
In addition, if both equations \eqref{drift_equation1_appendix} and \eqref{drift_equation2_appendix} hold, then the following is true
\begin{equation}
    \bE[\tau_m^C|\btheta_0=\hat{\btheta}]\leq V(\hat{\btheta})+(m-1)\sup_{\btheta\in C} V(\btheta).
\end{equation}
\end{lemma}
\begin{proof}
 See \cite{meyn2012markov}. 
\end{proof}
\subsection{Stopping Time Lemma}\label{stopping_time_lemma}
In light of drift equation \eqref{drift_equation_appendix}, the iterates are inclined towards the target set $C$. With a positive probability $\delta$, the test will be activated once we are in $C$. Hence, the expected value of the stopping time $T$, i.e. $\bE[T]$, can be upper-bounded in terms of $\delta$ and expected return times $\bE[\tau_m^C]$. 
\begin{lemma}\label{lem:stopping_time_appendix}
Suppose that $\bE[\tau_m^{C}]<\infty$ for all $m\geq 1$.  Then it is true that $T_C<+\infty$. Moreover, the following holds.
\begin{equation}\label{eq:ST_tctm}
   \bE[T]\leq \bE[T_C]\leq \sum_{m=1}^{\infty}\bE[\tau_m^{C}](1-\delta)^{m-1},
\end{equation}
where for any fixed $\btheta\in C$ the constant $\delta$ satisfies  
\begin{equation}
    \delta= \min \mathbb{P}_{\bxi \sim \mathcal{P}_*}\left(\bxi^T\btheta\geq 1 \right).
\end{equation}
\end{lemma}

\subsection{Basic Convex Analysis Lemma}
Here we state and prove two basic results from convex analysis that we used in the paper. 
\begin{lemma}\label{lem:convex_analysis_lemma}
Suppose that $g:\R^{\geq 0}\to \R$ is a convex function with a minimizer at $\rho^*>0$. Assume that $g$ is twice differentiable on the interval $[\tfrac{3}{4}\rho^*,\tfrac{5}{4}\rho^*]$. Moreover, assume that there exists a constant $r>0$ such that $g''(\rho)\geq r$ for all $\rho \in [\tfrac{3}{4}\rho^*,\tfrac{5}{4}\rho^*]$. Then it holds that
\begin{equation}\label{eq0:cvx_lemma}
    g(\rho)-g(\rho^*)\geq \frac{\rho^*r}{8}\vert \rho-\rho^*\vert \quad \text{for all $\rho \not\in [\tfrac{1}{2}\rho^*,\tfrac{3}{2}\rho^*]$}.
\end{equation}
\end{lemma}
\begin{proof}
First, assume that $\rho > \tfrac{3}{2}\rho^*$ holds. There exists  $\hat{\rho}\in [\rho^*,\tfrac{5\rho^*}{4}]$ such that 
\begin{equation}\label{eq1:cvx_lemma}
    g'(\rho^*+\frac{\rho^*}{4})=g'(\rho^*+\frac{\rho^*}{4})-g'(\rho^*)=\frac{\rho^*}{4}g''(\hat{\rho})\geq \frac{\rho^*r}{4},
\end{equation}
where we used that $g'(\rho^*)=0$. With the convexity of $g$, for any $\rho>\frac{3\rho^*}{2}$, we have 
\[
g(\rho)\geq g(\rho^*+\frac{\rho^*}{4})+g'(\rho^*+\frac{\rho^*}{4})(\rho-\frac{5\rho^*}{4})\geq g(\rho^*)+\frac{\rho^*r}{4}(\rho-\frac{5\rho^*}{4}).
\]
Note that the second inequality follows from \eqref{eq1:cvx_lemma} and the optimal value of $g$ occurring at $g(\rho^*)$. Using the identity, $2(\rho-\frac{5\rho^*}{4})\geq \frac{\rho^*}{4}+\rho-\frac{5\rho^*}{4}=\rho-\rho^*$, we conclude 
\begin{equation}\label{eq:cvx_lemma1}
    g(\rho)-g(\rho^*)\geq \tfrac{1}{8}\rho^*r(\rho-\rho^*) \quad \text{for all $\rho > \frac{3\rho^*}{2}$}.
\end{equation}
We now consider the second case, $\rho<\frac{\rho^*}{2}$. Similarly as above, we get 
\begin{equation}\label{eq2:cvx_lemma}
    -g'(\rho^*-\frac{\rho^*}{4})= g'(\rho^*)-g'(\rho^*-\frac{\rho^*}{4})=\frac{\rho^*}{4}g''(\hat{\rho})\geq \frac{\rho^*r}{4}.
    \end{equation}
    for some $\hat{\rho}\in [\frac{3\rho^*}{4},\rho^*]$. Since $\rho<\frac{\rho^*}{2}$, we have 
    \[
    g(\rho)\geq g(\rho^*-\frac{\rho^*}{4})+g'(\rho^*-\frac{\rho^*}{4})(\rho-\frac{3\rho^*}{4})\geq g(\rho^*)+\frac{\rho^*r}{4}(\frac{3\rho^*}{4}-\rho).
    \]
    Here, again, the first inequality follows from convexity of $g$ and the second inequality from \eqref{eq2:cvx_lemma} and $g(\rho^*-\frac{\rho^*}{4})\geq g(\rho^*)$. We note that $2(\frac{3\rho^*}{4}-\rho)\geq \frac{\rho^*}{4}+\frac{3\rho^*}{4}-\rho=\rho^*-\rho$ and therefore 
    \begin{equation}\label{eq:cvx_lemma2}
        g(\rho)-g(\rho^*) \geq \frac{\rho^*r}{8}(\rho^*-\rho)\quad \text{for all $\rho < \frac{\rho^*}{2}$}.
    \end{equation}
    Combining \eqref{eq:cvx_lemma1} and \eqref{eq:cvx_lemma2} the result follows. 
\end{proof}
We used the following technical lemma in the paper as well.
\begin{lemma}\label{lem:technical_convex_bound}
Consider the following optimization problem 
\[
\min f(\btheta):=\bE_{(\bxi,y)\sim \mathcal{P}_*}\left[\ell(\bxi^T\btheta)\right].
\]
where $\ell$ is a convex function. The sequences $\{\bm{\theta}_k, \bm{\xi}_k \}_{k = 0}^\infty$ generated by Algorithm~\ref{alg:SGD_termination} satisfy for any $\bm{\theta} \in \R^d$, the following
    \begin{equation} \label{eq:high_decrease}
       f(\bm{\theta}_{k-1})-f(\bm{\theta})\leq \frac{1}{2\alpha}\left(\Vert  \bm{\theta}_{k-1}-\bm{\theta} \Vert^2-\bE\left[\Vert \bm{\theta}_{k}-\bm{\theta} \Vert^2\, |\mathcal{F}_{k-1}\right] \right)+\bE[\Vert\nabla_{\btheta}\ell\left( \bxi_k^T\btheta\right)\Vert^2 \, | \, \mathcal{F}_{k-1}],
    \end{equation}
    for all $k\geq 1$ where $f$ is defined in \eqref{optimization_problem} and the filtration $\{\mathcal{F}_k\}_{k=0}^{+\infty}$ in \eqref{eq:sigma}.
\end{lemma}
\begin{proof}%[Proof of Lemma \ref{lem:high_tech}]
 Define the quantity 
  \begin{equation*}
      \bm{g_k}:=\frac{1}{\alpha}\left( \bm{\theta_{k-1}}-\bm{\theta_{k}}\right) = \nabla_{\btheta}\ell\left(\bxi_k^T\btheta \right). \end{equation*}
      Therefore, we obtain that 
      \[
      \bE_{\bxi_{k}}\left[\bm{g}_k|\mathcal{F}_{k-1} \right]=\nabla_{\btheta} f(\btheta_{k-1})
      \]
By convexity of the function $f$, we have for any $\bm{\theta} \in \R^d$ the following
\begin{align*}
\norm{\bm{\theta}_{k}-\bm{\theta}}^2 &= \norm{\bm{\theta}_{k-1}-\bm{\theta}}^2 -2 \alpha \bm{g}_k^T (\bm{\theta}_{k-1}-\bm{\theta}) + \alpha^2\norm{\bm{g}_k}^2\\
&= \norm{\bm{\theta}_{k-1}-\bm{\theta}}^2 - 2\alpha(\bm{g}_k-\bE_{\bxi_{k}}\left[\bm{g}_k|\mathcal{F}_{k-1} \right])^T(\bm{\theta}_{k-1}-\bm{\theta}) - 2 \alpha \bE_{\bxi_{k}}\left[\bm{g}_k|\mathcal{F}_{k-1} \right]^T (\bm{\theta}_{k-1}-\bm{\theta})+\alpha^2 \norm{\bm{g}_k}^2\\
&\le \norm{\bm{\theta}_{k-1}-\bm{\theta}}^2- 2\alpha(\bm{g}_k-\bE_{\bxi_{k}}\left[\bm{g}_k|\mathcal{F}_{k-1} \right])^T(\bm{\theta}_{k-1}-\bm{\theta})-2\alpha (f(\bm{\theta}_{k-1})-f(\bm{\theta})) + \alpha^2 \norm{\bm{g}_k}^2.
  \end{align*}
%Here, the last inequality follows from the Jensen's inequality.  
By taking conditional expectations with respect to $\mathcal{F}_{k-1}$ and rearranging the above inequality, the result follows.
\end{proof}

% \bibliographystyle{plainnat}
% \bibliography{bib}
